# Supplementary material for: Abstractors and relational cross-attention: An inductive bias for explicit relational reasoning in Transformers
Source: arXiv:2304.00195 source file (2024-04-12)
Supplement: Supplementary file 1 [file appendix_additional_experiments.tex]

\section{Additional Experiments}

\input{appendix/appendix_object_sorting_robustness.tex}
